# Supplementary material for: Semantic Composition in Visually Grounded Language Models
Source: arXiv:2305.16328 source file (2023-05-15)
Supplement: Supplementary file 1 [file Appendix_A.tex]

% An appendix
%======================================================================
\chapter*{Appendices}

% \chapter{Proof of Concept}
% \label{appA}
